# Supplementary material for: Toward Motion Robustness: A masked attention regularization framework in remote photoplethysmography
Source: arXiv:2407.06653 source file (2024-07-09)
Supplement: Supplementary file 1 [file X_suppl.tex]

\clearpage
\setcounter{page}{1}
\setcounter{section}{0}
\maketitlesupplementary

\section{Metric details}
We follow the approach outlined in \cite{Alpher34} by using mean absolute error (MAE), root mean square error (RMSE), mean absolute percentage error (MAPE), and Pearson’s correlation coefficient (r) as evaluation metrics for heart rate (HR). The details of related equations are as follows.
\begin{equation}
  MAE = \frac{1}{N} \sum_{n=1}^{N} \left| Z-Y \right|
  \label{eq:mae}
\end{equation}

\begin{equation}
  RMSE = \sqrt{\frac{1}{N} \sum_{n=1}^{N}(Z-Y)^{2}}
  \label{eq:rmse}
\end{equation}

\begin{equation}
  MAPE = \frac{1}{N} \sum_{n=1}^{N} \left| \frac{Z-Y}{Z} \right|
  \label{eq:mape}
\end{equation}

\begin{equation}
  \small r =\frac{\sum_{n=1}^{N}(Z_{n}-\overline{Z})(Y_{n}-\overline{Y})}{\sqrt{(\sum_{n=1}^{N}Z_{n}-\overline{Z})^{2}(\sum_{n=1}^{N}Y_{n}-\overline{Y})^{2}}}
  \label{eq:pearson}
\end{equation}

\section{Ablation study}
\label{sec:ablation}

\subsection{HRV and RF evaluation}  

The face is a complex structure that contains numerous blood vessels, which play a crucial role in maintaining the health and function of the skin and underlying tissues. Fig.~\ref{fig8} is an overview of the distribution of blood vessels in the face. The facial veins are located just beneath the skin and drain blood from the surface of the face, running throughout forehead, cheek, chin, eyebrow, and nose. The alteration in light absorption resulting from blood flow is crucially significant for rPPG measurements. Our novel approach, MAR-rPPG, is designed to capture these variations and provide precise heart rate assessments.

Following the method \cite{Alpher33}, we evaluate the heart rate variability (HRV) and respiratory frequency (RF) performance of our proposed MAR-rPPG on the UBFC-rPPG dataset. For HRV, we assess three attributes: the low frequency (LF), high frequency (HF), and LF/HF ratio, and LF and HF are determined using the interbeat intervals in the low-frequency (0.04 to 0.15 Hz) and high-frequency (0.15 to 0.4 Hz) ranges of rPPG signals. To comprehensively report the performance, we utilize three metrics: standard deviation (Std), RMSE, and Pearson's correlation coefficient $r$. We conduct a five-fold cross-validation experiment and compare our approach with some famous methods, such as POS \cite{Alpher22}, CHROM \cite{Alpher08}, GREEN \cite{Alpher09}, CVD \cite{Alpher25}, rPPGNet \cite{Alpher26}, Dual-Gan \cite{Alpher46}, Physformer \cite{Alpher27}, Gideon \etal \cite{Alpher51}, REA-LFA \cite{Alpher33}. We utilize the toolkit HeartPy \cite{Alpher52} to calculate HRV and RF.

As shown in Tab.~\ref{tab2}, we can see that MAR-rPPG surpasses all traditional ones and many deep learning ones. Besides, our approach offers improved accuracy in estimating RF and LF/HF ratio when compared to other advanced methods. For LF and HF, PhysFormer and Dual-GAN show better performance. This suggests that the proposed technique has the potential to excel not only in heart rate estimation tasks but also in predicting rPPG signals for RF measurements and heart rate variability analysis.

\begin{figure}[t]
    \begin{center}
    \includegraphics[width=2.6in]{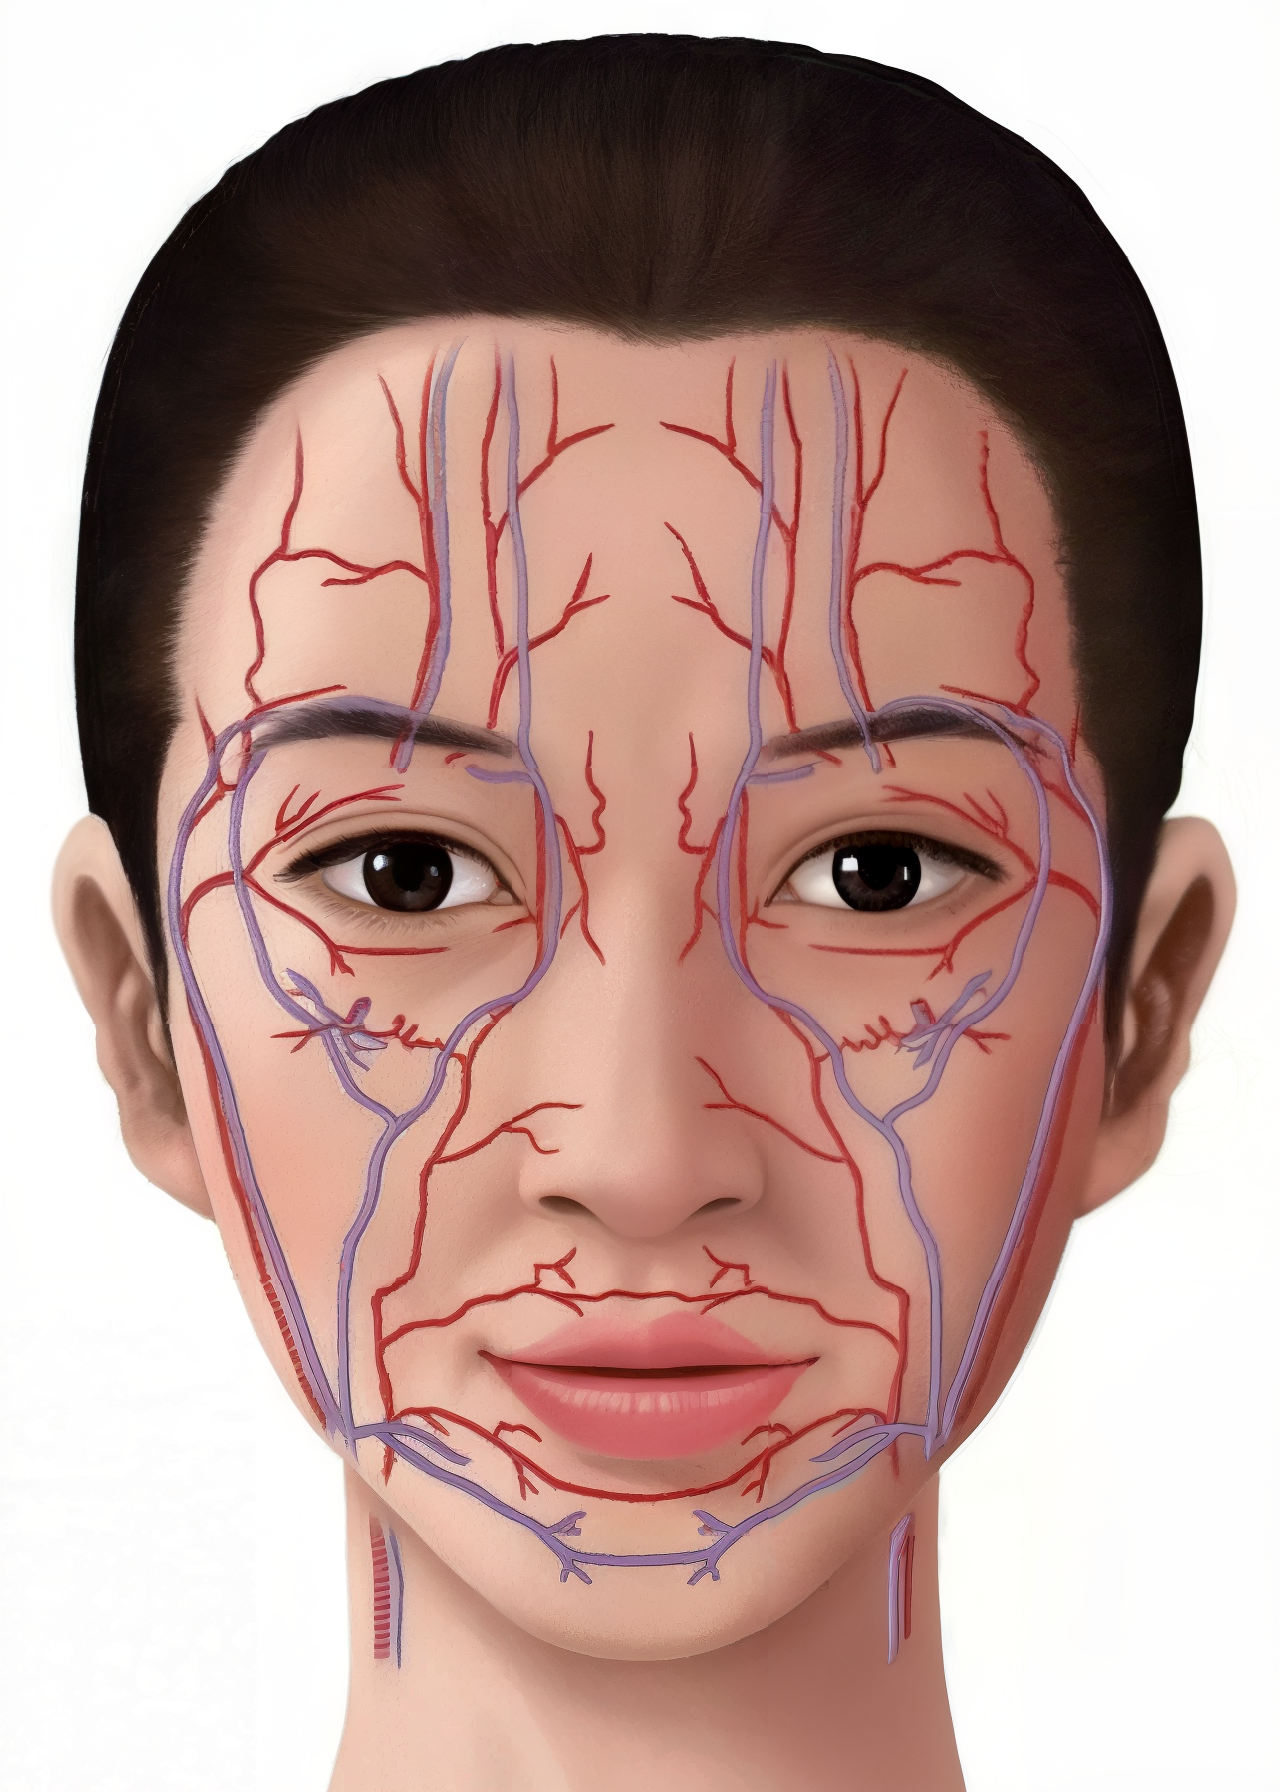} \\
    \end{center}
    \vspace{-0.1in}
    \caption{The overview of superficial facial veins.}
    \label{fig8}
  \end{figure}

% \begin{figure}[t]
%     \begin{center}
%     \begin{tabular}{cc}
%     \includegraphics[width=3.2in]{figs/wave_subject33_L3_MO3_E2_S3_GE2_GL2_H2_MA2.png} \\
%     \scriptsize (a) Talking sample\\
%     \includegraphics[width=3.2in]{figs/wave_subject33_L4_MO4_E2_S3_GE2_GL2_H2_MA2.png} \\
%     \scriptsize (b) Walking sample\\
%     \end{tabular}
%     \end{center}
%     \vspace{-0.1in}
%     \caption{The estimated rPPG signals on talking and walking motion samples of MMPD dataset. }
%     \label{fig7}
%   \end{figure}

\begin{table*}[!t]
    \vspace{-0.1in}
    \begin{center}
    \setlength{\tabcolsep}{1mm}
    \begin{tabular}{c|ccc|ccc|ccc|ccc}
    \toprule
    % &&&&&\multicolumn{9}{c}{} \\ 
    \multirow{2}*{Method} &\multicolumn{3}{c|}{RF}& \multicolumn{3}{c|}{HRV: LF}& \multicolumn{3}{c|}{HRV: HF}& \multicolumn{3}{c}{HRV: LF/HF}\\
    
    &Std$\downarrow$  &RMSE$\downarrow$  &$r\uparrow$  & Std$\downarrow$  &RMSE$\downarrow$  &$r\uparrow$ & Std$\downarrow$  &RMSE$\downarrow$  &$r\uparrow$ & Std$\downarrow$  &RMSE$\downarrow$  &$r\uparrow$\\ 
    \midrule
    POS \cite{Alpher22} &0.109  &0.107  &0.087  &0.171  &0.169  &0.479  &0.171  &0.169  &0.479 &0.405 &0.399 &0.518\\
    CHROM \cite{Alpher08} &0.086  &0.089  &0.102  &0.243  &0.240  &0.159 &0.243  &0.240  &0.159 &0.655 &0.645  &0.266\\
    GREEN \cite{Alpher09} &0.087  &0.086  &0.111  &0.186  &0.186  &0.280  &0.186  &0.186  &0.280 &0.361 &0.365  &0.492\\
    CVD \cite{Alpher25}   &0.017  &0.018  &0.252  &0.053  &0.065 &0.740  &0.053  &0.065  &0.740 &0.169 &0.168  &0.812\\
    rPPGNet \cite{Alpher26} &0.030  &0.034  &0.233  &0.071 &0.070 &0.686  &0.071  &0.070 &0.686 &0.212 &0.208  &0.744\\
    Dual-Gan \cite{Alpher46}  &0.010  &0.010  &0.395  &0.034 &0.035  &0.891  &0.034  &0.035  &0.891 &0.131 &0.136  &0.881\\
    Physformer \cite{Alpher27}  &0.009  &\textbf{0.009}  &0.413  &\textbf{0.030} &\textbf{0.032} &\textbf{0.895}  &\textbf{0.030} &\textbf{0.032} &\textbf{0.895} &0.126 &0.130  &0.893\\
    Gideon \etal \cite{Alpher51}  &0.061  &0.098  &0.103  &0.091  &0.139  &0.694  &0.091  &0.139  &0.694  &0.525 &0.691  &0.684\\
    REA-LFA \cite{Alpher33} &0.023  &0.028  &0.351  &0.047  &0.062  &0.769  &0.047 &0.062  &0.769 &0.160 &0.164  &0.831 \\ 
    \midrule
    MAR-rPPG(Ours)  &\textbf{0.008}  &0.031  &\textbf{0.838}  &0.065  &0.283  &0.856   &0.065  &0.283  &0.856 &\textbf{0.029} &\textbf{0.126}  &\textbf{0.925}\\ 
    
    \bottomrule
    \end{tabular}
    \end{center}
    \caption{Comparison of RF and HRV estimations on the UBFC-rPPG dataset. The best results are in bold. Std: standard deviation, RMSE: Root Mean Square Error, r: Pearson correlation coefficient.}
    \label{tab2}
\end{table*}

\subsection{Loss hyperparameter selection}

As illustrated in Tab.~\ref{tab5}, we can find that the hyperparameter $\alpha$ and $\beta$ are retain consistant and accurate rPPG estimation on the PURE dataset, while only one parameter setting with $\alpha = 0.1$ and $\beta = 0.9$ cannot converge and no metric outputs. We select $\alpha = 0.3$ and $\beta = 0.5$ for all experiments in this paper.

\begin{table*}[!t]
    \vspace{-0.1in}
    \begin{center}
    \setlength{\tabcolsep}{1mm}
    \begin{tabular}{c|c|cccc}
    \toprule
    
    $\alpha$  & $\beta$  & MAE $\downarrow$  &RMSE$\downarrow$ &MAPE$\downarrow$ &$r\uparrow$\\ 
    \midrule
    0.1  &0.1  &0.250 &0.645 &0.273 &1.000\\
    0.1  &0.3  &0.083 &0.288 &0.106 & 1.000\\
    0.1  &0.5  &0.083 &0.288 &0.106 & 1.000\\
    0.1  &0.7  &0.083 &0.288 &0.106 & 1.000\\
    0.1  &0.9  & - & - & - & -\\
    0.3  &0.1  &0.166 &0.408 &0.267 &1.000\\
    0.3  &0.3  &0.250 &0.865 &0.324 &0.999\\
    \colorbox{gray!50}{0.3}  &\colorbox{gray!50}{0.5}  &\colorbox{gray!50}{0.083} &\colorbox{gray!50}{0.288} &\colorbox{gray!50}{0.106} & \colorbox{gray!50}{1.00}\\
    0.3  &0.7  &0.333  &0.706 &0.440 &0.999\\
    0.3  &0.9  &0.083 &0.288 &0.106  & 1.000\\
    0.5  &0.1  &0.083 &0.288 &0.106  & 1.000\\
    0.5  &0.3  &0.083 &0.288 &0.106  & 1.000\\
    0.5  &0.5  &0.083 &0.288 &0.106  & 1.000\\
    0.5  &0.7  &0.083 &0.288 &0.106 & 1.000\\
    0.5  &0.9  &0.083 &0.288 &0.106  & 1.000\\
    0.7  &0.1  &0.166  &0.577 &0.166 &1.000\\
    0.7  &0.3  &0.083 &0.288 &0.106  & 1.000\\
    0.7  &0.5  &0.083 &0.288 &0.159 & 1.000\\
    0.7  &0.7  &0.083 &0.288 &0.106  & 1.000\\
    0.7  &0.9  &0.083 &0.288 &0.106  & 1.000\\
    0.9  &0.1  &0.166  &0.577 &0.166 &1.000\\
    0.9  &0.3  &0.083 &0.288 &0.106  & 1.000\\
    0.9  &0.5  &0.166  &0.577 &0.166  &1.000\\
    0.9  &0.7  &0.083 &0.288 &0.106  & 1.000\\
    0.9  &0.9  &0.083 &0.288 &0.106  & 1.000\\
    
    \bottomrule
    \end{tabular}
    \end{center}
    \caption{Ablation study for loss hyperparameter $\alpha$ and $\beta$. Our implementation is marked in \colorbox{gray!50}{shadow}, `-' indicates that the relavant parameters cannot converge.}
    \label{tab5}
\end{table*}
